# Supplementary material for: TeGA: Texture Space Gaussian Avatars for High-Resolution Dynamic Head Modeling
Source: arXiv:2505.05672 source file (2025-05-08)
Supplement: Supplementary file 2 [file A-Appendix.tex]

\subsection{Scene Scaling}
- As we use positionally encoded MLPs and gaussian densifications, two factors are desireable
- For 3DGS densification, ideally the scene as a whole should approximately span [-1,1]
- For human faces, this makes a scale of 1 dm = 1 unit ideal
- Human face is roughly 2 decimeters wide
- Human face surface when unwrapped is roughly 5 dm wide, spanning [0,1] in UV space 
- We use a scale factor of 5 for the depth, to ensure that gaussians moving horizontally and vertically in UVD space approximately moves similar amounts of distance
