# Supplementary material for: TeGA: Texture Space Gaussian Avatars for High-Resolution Dynamic Head Modeling
Source: arXiv:2505.05672 source file (2025-05-08)
Supplement: Supplementary file 5 [file 99-macros.tex]

\usepackage{xfrac}
%\usepackage{float}
\usepackage{soul}
%\usepackage{stfloats}

%% author comments
\newcommand{\AM}[1]{{\color{blue}[AM: #1]}}
\newcommand{\tb}[1]{{\color{magenta}[TB: #1]}}
\newcommand{\SL}[1]{{\color{purple}[SL: #1]}}
\newcommand{\KS}[1]{{\color{teal}[KS: #1]}}
\newcommand{\PG}[1]{{\color{orange}[PG: #1]}}
\newcommand{\AL}[1]{{\color{olive}[AL: #1]}}
\newcommand{\todo}[1]{{\color{red}[TODO: #1]}}
\newcommand{\SJG}[1]{{\color{violet}[SJG: #1]}}
%% disable author comments by commenting this in:
% \newcommand{\AM}[1]{}
% \newcommand{\TB}[1]{}
% \newcommand{\fm}[1]{}
% \newcommand{\SL}[1]{}
% \newcommand{\KS}[1]{}
% \newcommand{\MB}[1]{}
% \newcommand{\oh}[1]{}
% \newcommand{\tb}[1]{}

\definecolor{lightred}{RGB}{237.,146.,191.}

\definecolor{lightorange}{RGB}{255.0,176.0,127.0 }

\definecolor{lightyellow}{RGB}{255.0,215.0,127.0}

% \newcommand{\hlred}[1]{{\sethlcolor{lightred}\hl{#1}}}
% \newcommand{\hlorange}[1]{{\sethlcolor{lightorange}\hl{#1}}}
% \newcommand{\hlyellow}[1]{{\sethlcolor{lightyellow}\hl{#1}}}

\DeclareRobustCommand{\hlredcaption}[1]{{\sethlcolor{lightred}\hl{#1}}}
\DeclareRobustCommand{\hlorangecaption}[1]{{\sethlcolor{lightorange}\hl{#1}}}
\DeclareRobustCommand{\hlyellowcaption}[1]{{\sethlcolor{lightyellow}\hl{#1}}}

\newcommand{\hlred}[1]{\cellcolor{lightred}{#1}}
\newcommand{\hlorange}[1]{\cellcolor{lightorange}{#1}}
\newcommand{\hlyellow}[1]{\cellcolor{lightyellow}{#1}}

\newcommand{\rev}[1]{{\color{red} #1}}

\newcommand{\expressionnumber}{30}

\newcommand{\oursname}{OURSNAME\xspace}
\newcommand{\nerfname}{NeRF-SHL\xspace}

\newcommand{\eg}{\emph{e.g.}}
\newcommand{\ie}{\emph{i.e.}}
\newcommand{\etal}{\emph{et~al.}}

% Fig/Tab shortcut
\newcommand{\reffig}[1]{Fig.~\ref{#1}}
\newcommand{\reftab}[1]{Table~\ref{#1}}
\newcommand{\refeq}[1]{Eq.~\ref{#1}}
\newcommand{\refsec}[1]{Sec.~\ref{#1}}
\newcommand{\ccite}[1]{~\cite{#1}}

% Paragraph headings for related work 
\newcommand{\myparagraph}[1]{\vskip 0.5em\noindent\textbf{#1.}}
% Comments for last minute editing (can be easily hidden)
% Usage
% \hiddencomment{TEST}
% \suppcomment{TEST}
% \editcomment{TEST}
\newcommand{\showcomments}{false} % Hide by setting to false
\newcommand{\hiddencomment}[1]{\iftrue {\color{gray}#1}\else {}\fi}  
\newcommand{\suppcomment}[1]{\iftrue {\color{red}[move to supp:] #1}\else {}\fi}  
\newcommand{\editcomment}[1]{\iftrue {\color{green}[edit:] #1}\else {}\fi}  

%\DeclareMathOperator*{\mmin}{min}
%\DeclareMathOperator*{\mmax}{max}
%\DeclareMathOperator{\Tr}{Tr}
\newcommand{\abs}[1]{\left\lvert#1\right\rvert}
\newcommand{\norm}[1]{\left\lVert#1\right\rVert}
\newcommand{\x}[0]{\mathbf{x}}
\newcommand{\wi}[0]{\omega_i}
\newcommand{\wo}[0]{\omega_o}
